# Supplementary material for: Efficient Symptom Inquiring and Diagnosis via Adaptive Alignment of Reinforcement Learning and Classification
Source: arXiv:2112.00733 source file (2022-06-05)
Supplement: Supplementary file 1 [file coverletter.tex]

%%%% ijcai22.tex

\typeout{IJCAI--22 Instructions for Authors}

% These are the instructions for authors for IJCAI-22.

\documentclass{article}
\pdfpagewidth=8.5in
\pdfpageheight=11in
% The file ijcai22.sty is NOT the same as previous years'
\usepackage{ijcai22}

% Use the postscript times font!
\usepackage{times}
\usepackage{soul}
\usepackage{url}
\usepackage[hidelinks]{hyperref}
\usepackage[utf8]{inputenc}
\usepackage[small]{caption}
\usepackage{graphicx}
\usepackage{amsmath}
\usepackage{amsthm}
\usepackage{booktabs}
\usepackage{algorithm}
\usepackage{algorithmic}
\urlstyle{same}

% the following package is optional:
%\usepackage{latexsym}

% See https://www.overleaf.com/learn/latex/theorems_and_proofs
% for a nice explanation of how to define new theorems, but keep
% in mind that the amsthm package is already included in this
% template and that you must *not* alter the styling.
\newtheorem{example}{Example}
\newtheorem{theorem}{Theorem}

% Following comment is from ijcai97-submit.tex:
% The preparation of these files was supported by Schlumberger Palo Alto
% Research, AT\&T Bell Laboratories, and Morgan Kaufmann Publishers.
% Shirley Jowell, of Morgan Kaufmann Publishers, and Peter F.
% Patel-Schneider, of AT\&T Bell Laboratories collaborated on their
% preparation.

% These instructions can be modified and used in other conferences as long
% as credit to the authors and supporting agencies is retained, this notice
% is not changed, and further modification or reuse is not restricted.
% Neither Shirley Jowell nor Peter F. Patel-Schneider can be listed as
% contacts for providing assistance without their prior permission.

% To use for other conferences, change references to files and the
% conference appropriate and use other authors, contacts, publishers, and
% organizations.
% Also change the deadline and address for returning papers and the length and
% page charge instructions.
% Put where the files are available in the appropriate places.

% PDF Info Is REQUIRED.
% Please **do not** include Title and Author information
\pdfinfo{
/TemplateVersion (IJCAI.2022.0)
}

\title{Efficient Symptom Inquiring and Diagnosis via Adaptive Alignment of Reinforcement Learning and Classification}

% Single author syntax
\author{
    Submitted to AAAI 2022 Main Track and rejected in Phase 2\\
    Submission ID: 3519
}

% Multiple author syntax (remove the single-author syntax above and the \iffalse ... \fi here)
% Check the ijcai22-multiauthor.tex file for detailed instructions
\iffalse
\author{
First Author$^1$
\and
Second Author$^2$\and
Third Author$^{2,3}$\And
Fourth Author$^4$
\affiliations
$^1$First Affiliation\\
$^2$Second Affiliation\\
$^3$Third Affiliation\\
$^4$Fourth Affiliation
\emails
\{first, second\}@example.com,
third@other.example.com,
fourth@example.com
}
\fi

\begin{document}

\maketitle

\section{Summary of Paper Reviews}

After the review procedure of AAAI 2022, our previous submission was only reviewed by 3 reviewers (which should have been 4). All the reviewers claimed that our submission was good in technical soundness, reproducibility and clear writing. 

\vspace{0.8cm}
\textbf{The reasons to accept} is mainly summarized as follows:
\begin{enumerate}
    \item Our paper is well-written with clear motivation and technical details presentations.
    \item The proposed method is powerful and achieves state-of-the-art results on several datasets.
    \item We propose a new dataset with more diseases and more comprehensive information for synthetic patient simulation, where there is increasing value for the research community.
\end{enumerate}

\textbf{The reasons to reject} is mainly summarized as follows:
\begin{enumerate}
    \item Proposing a novel dataset is one of our contribution, while the details of the proposed dataset is not enough.
    \item There are concerns of lack of novelty for our proposed dataset. The key novelty of our proposed dataset is the adaptive threshold, while the descriptions of this part and the corresponding experiments are not enough.
    \item We do not provide the variance of the experiments, which makes our result less credible. 
    \item We do not provide how the hyper-parameters of our method are determined.
    \item One reviewer thinks the automatic diagnosis task can be solved by supervised sequential systems like LSTM or GRUs, and there is no need for reinforcement learning methods.
\end{enumerate}

\vspace{0.8cm}
The meta reviewer gave a rejection in consideration of the lack of novelty and few details of the proposed dataset. 

\section{The Changes Made}

To address the reviewers' comments, we summarize our changes as follows:
\begin{enumerate}
    \item As for the proposed dataset, the former version of our proposed dataset is constructed using MedType to extract entities from MedlinePlus articles. In this submission, we use BIOS\footnote{https://bios.idea.edu.cn/} vocabulary to generate the new version of the dataset with higher quality by maximum forward matching.
    \item We provide the basic statistics, examples, and the construction procedure of our proposed dataset in the technical supplementary material to help the reviewers thoroughly understand our dataset.
    \item One reviewer gave us a very constructive comment that we could set exclusive adaptive thresholds for each disease. We modify our method according to the reviewer's suggestion. The adaptive threshold is not unified across diseases, and the thresholds are different for each disease.
    \item We rewrite the method part of the paper and give more details of our method. We also design additional experiments to illustrate the effectiveness of our method.
    \item We provide the variance of the result of our method. The low variance indicates that the superior performance is not accidental.
    \item We provide more experimental details such as how the hyper-parameters are determined in the technical supplementary.
\end{enumerate}


\section{Full Reviews from Former Submission}

\subsection{Reviewer 1}

1. \textbf{Summary} Please briefly summarize the main claims/contributions of the paper in your own words. (Please do not include your evaluation of the paper here).\\
This work deals with the task of medical diagnosis through a series of symptom inquiries. The task is decomposed into two parts, the symptom-inquiring that is framed as an MDP requiring RL methods, and the disease diagnosing that is framed as a classification task. The main contributions are the adaptive entropy threshold as a stopping criterion for symptom-inquiring phase (and subsequently a diagnosis from the classifier is provided), and the newly collected synthetic dataset. Experiments on two synthetic datasets show that the proposed method outperforms baselines from prior work.

2. \textbf{Novelty} How novel are the concepts, problems addressed, or methods introduced in the paper?\\
Fair: The paper contributes some new ideas.

3. \textbf{Soundness} Is the paper technically sound?\\
Good: The paper appears to be technically sound, but I have not carefully checked the details.

4. \textbf{Impact} How do you rate the likely impact of the paper on the AI research community?\\
Good: The paper is likely to have high impact within a sub-field of AI OR moderate impact across more than one sub-field of AI.

5. \textbf{Clarity} Is the paper well-organized and clearly written?\\
Fair: The paper is somewhat clear, but some important details are missing or unclear.

6. \textbf{Evaluation} If applicable, are the main claims well supported by experiments?\\
Good: The experimental evaluation is adequate, and the results convincingly support the main claims.

7. \textbf{Resources} If applicable, how would you rate the new resources (code, data sets) the paper contributes? (It might help to consult the paper’s reproducibility checklist)\\
Good: The shared resources are likely to be very useful to other AI researchers.

8. \textbf{Reproducibility} Are the results (e.g., theorems, experimental results) in the paper easily reproducible? (It may help to consult the paper’s reproducibility checklist.)\\
Good: key resources (e.g., proofs, code, data) are available and key details (e.g., proofs, experimental setup) are sufficiently well-described for competent researchers to confidently reproduce the main results.

9. \textbf{Ethical Considerations} Does the paper adequately address the applicable ethical considerations, e.g., responsible data collection and use (e.g., informed consent, privacy), possible societal harm (e.g., exacerbating injustice or discrimination due to algorithmic bias), etc.?\\
Not Applicable: The paper does not have any ethical considerations to address.

10. \textbf{Reasons to Accept} Please list the key strengths of the paper (explain and summarize your rationale for your evaluations with respect to questions 1-9 above).\\
The paper is well-written with clear motivation and contributions, and the solution seems well-designed.
Results over SoTA baselines show that the proposed method performs well.
Code and data are available (assuming that both will be open-sourced, there is increased value for the research community).

11. \textbf{Reasons to Reject} Please list the key weaknesses of the paper (explain and summarize your rationale for your evaluations with respect to questions 1-9 above).\\
The details provided on the new dataset are very limited. Since the dataset is a novel contribution, there should be sufficient details for subsequent works to understand the data and its limitations. For example, bar plots or other forms to pictorially describe the data distribution need to be added in the supplementary.

Compared to prior work, apart from the dataset, it seems that the main difference lies in the stopping criterion but this section is relatively unexplained. For example, what is the dynamic threshold K and how is it set? Does it refer to an initial value set for K? 

Most ideas in this paper originate from entropy regularization, reward design and uncertainty estimation. Seems technically solid, but limited novelty in terms of methodology.


12. \textbf{Questions for the Authors} Please provide questions that you would like the authors to answer during the author feedback period. Please number them.\\
How is the dynamic threshold set?

Have you tried other fixed thresholds? It seems that the best dynamic threshold is too small compared to the predefined fixed values in Table 1 (Appendix). How do results looks like when the fixed threshold is close to 0.1 or 0.01? Is there any prior knowledge that could be leveraged to set this threshold for example? 

How about other forms of scheduling or uncertainty estimation?

13. \textbf{Detailed Feedback for the Authors} Please provide other detailed, constructive, feedback to the authors.\\
Consider reporting average and standard deviation over a fixed set of trials. Especially for the ablation studies, where results between methods exhibit a small margin, adding standard deviation might provide more insights.

There are no details about the two network architectures. 

Typos:
- Medical automatic diagnosis (MAD) or dialogue systems
for medical automatic diagnosis (DSMAD) is one of $-->$ are two of

- are only tested on dataset containing few disease $-->$ on a dataset (or datasets) containing a few diseases

14. \textbf{OVERALL EVALUATION} Please provide your overall evaluation of the paper, carefully weighing the reasons to accept and the reasons to reject the paper. Ideally, we should have: - No more than 25\% of the submitted papers in (Accept + Strong Accept + Very Strong Accept + Award Quality) categories; - No more than 20\% of the submitted papers in (Strong Accept + Very Strong Accept + Award Quality) categories; - No more than 10\% of the submitted papers in (Very Strong Accept + Award Quality) categories - No more than 1\% of the submitted papers in the Award Quality category\\
Weak Accept: Technically solid, moderate to high impact paper, with no major concerns with respect to evaluation, resources, reproducibility, ethical considerations.



\subsection{Reviewer 2}

1. \textbf{Summary} Please briefly summarize the main claims/contributions of the paper in your own words. (Please do not include your evaluation of the paper here).\\
This paper proposed a novel framework for medical automatic diagnosis (MAD). 
This framework consists of two parts: 
1. A Symptom-Inquiring agent using a policy network aims to generate efficient and large information inquiring. \\
2. Disease-Diagnosing Model decides whether an additional inquiring is needed or not via the entropy thresholds, then diagnoses the disease.\\
In my opinion, the contributions of this paper are as follows:\\
1. the entropy threshold is adaptive, which shows good performances and robustness in experiments.\\
2. This paper generated few new datasets with more diseases and symptoms to simulate synthetic patients.\\
3. The method proposed in this paper shows very good performance in MAD tasks.

2. \textbf{Novelty} How novel are the concepts, problems addressed, or methods introduced in the paper?\\
Fair: The paper contributes some new ideas.

3. \textbf{Soundness} Is the paper technically sound?\\
Good: The paper appears to be technically sound, but I have not carefully checked the details.

4. \textbf{Impact} How do you rate the likely impact of the paper on the AI research community?\\
Fair: The paper is likely to have moderate impact within a subfield of AI.

5. \textbf{Clarity} Is the paper well-organized and clearly written?\\
Excellent: The paper is well-organized and clearly written.

6. \textbf{Evaluation} If applicable, are the main claims well supported by experiments?\\
Good: The experimental evaluation is adequate, and the results convincingly support the main claims.

7. \textbf{Resources} If applicable, how would you rate the new resources (code, data sets) the paper contributes? (It might help to consult the paper’s reproducibility checklist)\\
Good: The shared resources are likely to be very useful to other AI researchers.

8. \textbf{Reproducibility} Are the results (e.g., theorems, experimental results) in the paper easily reproducible? (It may help to consult the paper’s reproducibility checklist.)\\
Good: key resources (e.g., proofs, code, data) are available and key details (e.g., proofs, experimental setup) are sufficiently well-described for competent researchers to confidently reproduce the main results.

9. \textbf{Ethical Considerations} Does the paper adequately address the applicable ethical considerations, e.g., responsible data collection and use (e.g., informed consent, privacy), possible societal harm (e.g., exacerbating injustice or discrimination due to algorithmic bias), etc.?\\
Excellent: The paper comprehensively addresses all of the applicable ethical considerations.

10. \textbf{Reasons to Accept} Please list the key strengths of the paper (explain and summarize your rationale for your evaluations with respect to questions 1-9 above).\\
1. I think the adaptive entropy threshold is interesting and powerful, which shows good performances and robustness in experiments.
2. The paper is well written and the algorithm is descibled clearly in details . 
And I think the model is well designed, especially the rewards are reasonable. The algorithm has good performances in few datasets.
3. This paper generated few new datasets with more diseases and symptoms to simulate synthetic patients.

11. \textbf{Reasons to Reject} Please list the key weaknesses of the paper (explain and summarize your rationale for your evaluations with respect to questions 1-9 above).\\
1. The innovation of algorithm is not enough. The only innovation I think is the adaptive entropy threshold. Hence, more analysis of it is needed. e.g., Does the adaptive entropy threhold need more epoches for training? Why all diseases use one entropy threhold? \\
2. This method has more superparameters, how to determine the values of them.\\
3. The experiments are not enough. Do the results in the table 1 and 2 are only from one-time experiments? This makes the result unreliable because it may be accidental. And showing the variance can make the results more credible.\\

12. \textbf{Questions for the Authors} Please provide questions that you would like the authors to answer during the author feedback period. Please number them.\\
1. More analysis of the adaptive entropy threshold.\\
2. This method has more superparameters, how to determine the values of them, by validation datasets?\\
3. The experiments are not enough and the results are not credible.

13. \textbf{Detailed Feedback for the Authors} Please provide other detailed, constructive, feedback to the authors.\\
1. This method has more superparameters than others, how to determine the values of them? Please introduce in this paper.

14. \textbf{OVERALL EVALUATION} Please provide your overall evaluation of the paper, carefully weighing the reasons to accept and the reasons to reject the paper. Ideally, we should have: - No more than 25\% of the submitted papers in (Accept + Strong Accept + Very Strong Accept + Award Quality) categories; - No more than 20\% of the submitted papers in (Strong Accept + Very Strong Accept + Award Quality) categories; - No more than 10\% of the submitted papers in (Very Strong Accept + Award Quality) categories - No more than 1\% of the submitted papers in the Award Quality category\\
Borderline reject: Technically solid paper where reasons to reject, e.g., lack of novelty, outweigh reasons to accept, e.g., good evaluation. Please use sparingly.


\subsection{Reviewer 4\footnote{Missing Reviewer 3}}
1. \textbf{Summary} Please briefly summarize the main claims/contributions of the paper in your own words. (Please do not include your evaluation of the paper here).\\
This method proposes an RL + classification method starting from the patient's self-reported symptoms leading to (a) a symptom inquiring module that asks the (synthetic) patient for more symptoms and (b) a classifier that assigns a probability to the possible diseases based on the increasing list of symptoms. The paper shows better accuracy compared to previous methods in the field on two proposed datasets for simulating synthetic patients.

2. \textbf{Novelty} How novel are the concepts, problems addressed, or methods introduced in the paper?\\
Good: The paper makes non-trivial advances over the current state-of-the-art.

3. \textbf{Soundness} Is the paper technically sound?\\
Good: The paper appears to be technically sound, but I have not carefully checked the details.

4. \textbf{Impact} How do you rate the likely impact of the paper on the AI research community?\\
Fair: The paper is likely to have moderate impact within a subfield of AI.

5. \textbf{Clarity} Is the paper well-organized and clearly written?\\
Good: The paper is well organized but the presentation could be improved.

6. \textbf{Evaluation} If applicable, are the main claims well supported by experiments?\\
Fair: The experimental evaluation is weak: important baselines are missing, or the results do not adequately support the main claims.

7. \textbf{Resources} If applicable, how would you rate the new resources (code, data sets) the paper contributes? (It might help to consult the paper’s reproducibility checklist)\\
Fair: The shared resources are likely to be moderately useful to other AI researchers.

8. \textbf{Reproducibility} Are the results (e.g., theorems, experimental results) in the paper easily reproducible? (It may help to consult the paper’s reproducibility checklist.)\\
Excellent: key resources (e.g., proofs, code, data) are available and key details (e.g., proof sketches, experimental setup) are comprehensively described for competent researchers to confidently and easily reproduce the main results.

9. \textbf{Ethical Considerations} Does the paper adequately address the applicable ethical considerations, e.g., responsible data collection and use (e.g., informed consent, privacy), possible societal harm (e.g., exacerbating injustice or discrimination due to algorithmic bias), etc.?\\
Good: The paper adequately addresses most, but not all, of the applicable ethical considerations.

10. \textbf{Reasons to Accept} Please list the key strengths of the paper (explain and summarize your rationale for your evaluations with respect to questions 1-9 above).\\
- The paper introduces a novel RL + classification based system for accurate diagnosis of diseases from the symptoms. The method is well formulated balancing the amount of inquiries to the patient and accuracy of the diagnosis.\\
- The paper presents two extensive datasets for simulating the synthetic patients with large number of diseases and symptoms leading to extensive evaluations.

11. \textbf{Reasons to Reject} Please list the key weaknesses of the paper (explain and summarize your rationale for your evaluations with respect to questions 1-9 above).\\
- What is the need for RL in this task? I believe the sequential querying of the symptoms can be done with supervised sequential decision making frameworks (such as LSTM, GRU etc) with the constraint of limited number of inquiries in the loss function?\\
- I believe addition of more qualitative examples on how the previous methods failed to diagnose the correct disease after certain number of inquiries whereas the proposed method could detect it in limited inquiries would improve the claim of the paper.

12. \textbf{Questions for the Authors} Please provide questions that you would like the authors to answer during the author feedback period. Please number them.\\
- What is the action space of the symptom inquiring agent - is it a binary action space that decides whether to ask the synthetic patient for the next symptoms? 
( the example in the supplementary shows such an inquiry system)

- Have you compared with supervised sequential systems like LSTM or GRUs for this tasks and how does that compare to the RL setup?

13. \textbf{Detailed Feedback for the Authors} Please provide other detailed, constructive, feedback to the authors.\\
- Please add more details on qualititive evaluations on how different methods inquire about additional symptoms from the synthetic patient along with the corresponding entropy values, This will better help analyse the quality of the proposed method further.\\
- If possible, please increase the size of the text in tables 1, 2, and 3.

14. \textbf{OVERALL EVALUATION} Please provide your overall evaluation of the paper, carefully weighing the reasons to accept and the reasons to reject the paper. Ideally, we should have: - No more than 25\% of the submitted papers in (Accept + Strong Accept + Very Strong Accept + Award Quality) categories; - No more than 20\% of the submitted papers in (Strong Accept + Very Strong Accept + Award Quality) categories; - No more than 10\% of the submitted papers in (Very Strong Accept + Award Quality) categories - No more than 1\% of the submitted papers in the Award Quality category\\
Borderline accept: Technically solid paper where reasons to accept, e.g., novelty, outweigh reasons to reject, e.g., limited evaluation. Please use sparingly.


\subsection{Meta Reviewer 1}
\textbf{The first piece of comments is missing.}

\textbf{2. Summary of the discussion among PC members. Please note whether there is broad agreement among the reviewers regarding their overall ratings (in sentiment if not scores), and key strengths and weaknesses with respect to review criteria, and any major points of disagreement among reviewers.}\\
Though a new dataset for automatic diagnosis is valuable and the feedbacks have partially satisfied the reviewers' question, there is still a concern over the limited novelty in terms of the methodology.

\textbf{3. Reasons to accept the paper. Please list the key arguments for accepting the paper.}\\
1. All reviewers aggree that a new released dataset for automatic diagnosis with RL should be a contribution of this paper.

2. The solution is well presented and formulated.

\textbf{4. Reasons to reject the paper. Please list the key arguments for rejecting the paper.}\\
1. The main drawback is the lack of novelty. The main idea of this paper to use adaptive entropy threshold to replace fixed threshold proposed by an AAAI 2020 paper (Xia et al. 2020). All reviwers pointed out that the techincal novleity of this paper is limited.

2. Since the main contribution is the dataset, more explaination about how to collect the dataset and a detailed analysis is deserved. 



%% The file named.bst is a bibliography style file for BibTeX 0.99c
% \bibliographystyle{named}
\bibliography{draft}

\section{The Anonymized Version of the Rejected Paper}
\newpage
\newpage




\end{document}
