# Supplementary material for: Efficient Symptom Inquiring and Diagnosis via Adaptive Alignment of Reinforcement Learning and Classification
Source: arXiv:2112.00733 source file (2022-06-05)
Supplement: Supplementary file 2 [file rebuttal.tex]

%%%% ijcai22-multiauthor.tex
\pdfoutput=1
\typeout{authors example}

% These are the instructions for authors for IJCAI-22.

\documentclass{article}
\pdfpagewidth=8.5in
\pdfpageheight=11in
% The file ijcai22.sty is NOT the same as previous years'
\usepackage{ijcai22}

% Use the postscript times font!
% \usepackage{times}
% \renewcommand*\ttdefault{txtt}
% \usepackage{soul}
% \usepackage{url}
% \usepackage[hidelinks]{hyperref}
% \usepackage[utf8]{inputenc}
% \usepackage[small]{caption}
% \usepackage{graphicx}
% \usepackage{amsmath}
% \usepackage{booktabs}
\usepackage{times}
\usepackage{soul}
\usepackage{url}
\usepackage[hidelinks]{hyperref}
\usepackage[utf8]{inputenc}
\usepackage[small]{caption}
\usepackage{graphicx}
\usepackage{amsmath}
\usepackage{amsthm}
\usepackage{booktabs}
\usepackage{algorithm}
\usepackage{algorithmic}
\urlstyle{same}

% the following package is optional:
%\usepackage{latexsym}

% Following comment is from ijcai97-submit.tex:
% The preparation of these files was supported by Schlumberger Palo Alto
% Research, AT\&T Bell Laboratories, and Morgan Kaufmann Publishers.
% Shirley Jowell, of Morgan Kaufmann Publishers, and Peter F.
% Patel-Schneider, of AT\&T Bell Laboratories collaborated on their
% preparation.

% These instructions can be modified and used in other conferences as long
% as credit to the authors and supporting agencies is retained, this notice
% is not changed, and further modification or reuse is not restricted.
% Neither Shirley Jowell nor Peter F. Patel-Schneider can be listed as
% contacts for providing assistance without their prior permission.

% To use for other conferences, change references to files and the
% conference appropriate and use other authors, contacts, publishers, and
% organizations.
% Also change the deadline and address for returning papers and the length and
% page charge instructions.
% Put where the files are available in the appropriate places.

%PDF Info Is REQUIRED.
% Please **do not** include Title and Author information
\pdfinfo{
/TemplateVersion (IJCAI.2022.0)
}

\title{Efficient Symptom Inquiring and Diagnosis via Adaptive Alignment of Reinforcement Learning and Classification}
% \author{
%     %Authors
%     % All authors must be in the same font size and format.
%     Hongyi Yuan\textsuperscript{\rm 1, 2},
%     Sheng Yu\textsuperscript{\rm 1, 2}\thanks{Sheng Yu is the corresponding author.}\\
% }
% \affiliations{
%     %Afiliations
%     \textsuperscript{\rm 1} Center for Statistical Science, Tsinghua University, China\\
%     \textsuperscript{\rm 2} Department of Industrial Engineering, Tsinghua University, China\\
%     yuanhy20@mails.tsinghua.edu.cn, syu@tsinghua.edu.cn\\
%     % If you have multiple authors and multiple affiliations
%     % use superscripts in text and roman font to identify them.
%     % For example,
% %
% % See more examples next
% }
% \title{IJCAI--22 Example on typesetting multiple authors}

% \author{
% Hongyi Yuan$^1$ $^2$\and
% Sheng Yu$^1$ $^2$\footnote{Contact Author}\and\\
% \affiliations
% $^1$Center for Statistical Science, Tsinghua University, China\\
% $^2$Department of Industrial Engineering, Tsinghua University, China\\
% \emails
% yuanhy20@mails.tsinghua.edu.cn,
% syu@tsinghua.edu.cn
% }


\begin{document}


\section*{General Response}

\paragraph{Why not evaluate on real world data?}

In the field of automatic diagnosis research, real-world data is generally not accessible under the consideration of patients' privacy or the high cost of collecting data. A lack of real-world data is one of the most concerning problems in medical AI research. Therefore, we were compromised to use synthetic data to demonstrate the effectiveness of our proposed method as much previous research did. Despite the real-world condition would be much more complicated, our experiments on the synthetic data showed the effectiveness of our methods on a large number of diseases and corresponding symptoms where previous methods failed to achieve a decent diagnostic process as illustrated in Table 1 and 2 in the main text. 

The motivation of proposing a new dataset is to bridge the gap between synthetic data and real-world data where the existing data neither has a large disease set (only 4 or 5 diseases) nor contains the medical examination information. 

\paragraph{The discrepancy between synthetic and real-world experiments}

We follow previous work to evaluate MAD methods on the synthetic datasets. There is a clear gap between synthetic data and real-world data where real-world data may contain more noise and is more complicated. However, through synthetic data, we can also have a glimpse of the MAD method's performance, despite the synthetic task being easier. Our method shows good performance and stability those previous work did not achieve.



\section*{Reviewer 1}

\paragraph{Validate the proposed approach on a real-world dataset.} It is pity that we do not have access to the large-scale diagnostic data and follow the evaluation protocols of previous research to conduct experiments on synthetic datasets. Please refer to General Response for more justification.
\paragraph{Concerns on the techniques might not be new.} Recent previous work has proposed different methods to use RL and classification for auto-diagnosis, while the idea of our adaptive thresholding method is new. Our method emphasized the imperfect alignment of RL and classification in the previous work. Despite being simple and straight-forward, the proposed method shows a great improvement over the previous work.

\section*{Reviewer 2}


\paragraph{Some symptom terms and lab test variables in the dataset could be removed or be more in fine-grained levels.} In your example, blood tests and physical examinations are two widely used tests in the diagnostic process, which we think should be kept. We admit that the examination is not fine-grained and one examination can relate to various outcomes. We claim the contributions of the data are 1) large disease and symptom set and 2) firstly including examination information.

\paragraph{Not a type of sequential records of individualized patient cases and overstatement of the method.} For the diagnostic process, the sequential information can be viewed as the doctors' decision-making process and it is not necessary to contain sequential information within the patient symptoms. For the evaluation of our methods, we do not claim reliability of the methods through experiments and we show the reasonable diagnostic result through the case study. In the case study, we provide the step-wise entropy value and the proportion of each symptom existing in each disease. We can see a gradually decreasing entropy value and the proportion of each symptom, this may demonstrate the rational diagnostic process accomplished by our methods. In real clinical settings, our method should have superior performance over previous works. Please refer to General Response for more justification.

\section*{Reviewer 3}

For the English problem, we will correct it in the final revision. Auto-diagnosis as a sequential decision problem is not new, and we carefully reviewed recent advances in this field to provide a better view of the related research and fair method comparison.

\paragraph{Not including synthetic visual information} Synthesizing multi-modal data is another field of research in Medicine and is out of the scope of our work. We admit different modal data is critical to medical diagnoses such as MRIs or ECGs, and different modals of data can be introduced to our method with different representation learning methods substituting the policy and classifier networks. 

\paragraph{Did not distinguish the criticality of different diseases.} Learning disease-specific entropies can distinguish the criticality in a way that there exist some diseases that have large final entropy threshold meaning the disease is hard to give an accurate diagnosis.

\section*{Reviewer 4}

\paragraph{Under-optimized problem of baselines} We make lots of efforts to reproduce the previous work because there is no open-resourced code. We report the best results of our reproduced baselines. Our method also outperforms the previously reported results on the SymCat dataset. 

\paragraph{More insights on our method and sole RL methods} The medical diagnosis, as mentioned in the main texts, contains two parts of actions, acquiring symptoms, and giving the diagnosis. Giving diagnosis is the final decision of the diagnostic process and is naturally a classification problem. Using the sole RL method on the unified action space of the two, reward design can not explicitly distinguish the two parts of actions and will result in a large action space to explore. This will make it difficult for RL to learn an optimal policy. As the experiment illustrates, on the MedlinePlus dataset, the sole RL method REFUEL keep inquiring for symptom until the maximum step limitation and fail to give a diagnosis, this is because the patient may have multiple positive symptoms while only one disease. Gaining reward from positive symptoms is much easier than diagnosing. This will explain why the sole RL method is unsatisfying. 


% Our work is not properly treated in both phases of reviewing. Our work aims to emphasize the method alignment problem for auto-diagnosis systems and proposes an adaptive method for better alignment. However, most of the reviewers focus on the problem that our experiments are not conducted on a real dataset which in this field of research, a realistic dataset is not accessible due to privacy and cost concerns. Notable previous work also conducted experiments on synthetic data.  Lack of realistic data is a general problem in this field of research. This work should not have such low scores because of synthetic data. What's more, Reviewer 3 is ridiculous, he/she gives a Weak Reject because of "just not enough". And the concerns on synthetic visual data are totally off the point. He/She admits to being a non-expert in this domain and his/her review should be ignored. In summary,  we argue that the reviewers have erroneous views on our work, and our work is worth better scores and reviews.
\end{document}
